# Supplementary material for: Near-Optimal Bayesian Online Assortment of Reusable Resources
Source: arXiv:2512.06997 source file (2025-12-07)
Supplement: Supplementary file 1 [file appendix.tex]

\section{Omitted Technical Details of \Cref{sec:adversarial}}
\subsection{General Concave Penalty Functions: Proof of \Cref{thm:concave competitive ratio}/\Cref{prop:concave competitive ratio-iid}}
\label{sec:general penalty}
\label{app:general-penalty}
In this section,
we prove \Cref{prop:concave competitive ratio-iid}. As a corollary, this will also prove \Cref{thm:concave competitive ratio}, simply because the reverse and forward expected LP are equivalent programs when rental times are fixed over time (\Cref{remark:iid-fixed}). This result
extends the result of \citet{GNR-14}
for arbitrary concave penalty functions
from infinite rental time setting
to our setting (i.e., i.i.d.\ stochastic rental times), but the competitive ratio is measured against the optimal objective value of the reverse expected LP.
To this end, we follow a similar randomized primal-dual argument 
as in \Cref{thm:exponential competitive ratio} 
but with a more involved 
algorithmically constructed dual solution.
Specifically, we introduce a sub-problem termed as \emph{Interval Assignment Problem (IAP)},
and an algorithm to solve it. We use the solution produced by this algorithm as a guide 
to construct the dual solution. 

\begin{definition}[Interval Assignment Problem (IAP)]
\label{def:IAP}
Consider $n$ intervals $\{[a_1, b_1], \dots, [a_n, b_n]\}$ 
defined on $\R$, where 
interval $i$ is from $a_i$ to $b_i$
and 
$a_1 < a_2 < \dots < a_n$.
Let $\contain_i$ be a subset of $n$ intervals
which covers position $a_i$,
i.e., $\contain_i = \{j\in[n]: a_i \in [a_j, b_j]\}$
and $\containn_i$ be its size, i.e., $\containn_i = |\contain_i|$.
\emph{Interval Assignment Problem}
requires to construct
an assignment $\{\assign_1, \dots, \assign_n\}\in\mathbb{Z}_{\geq 0}^n$ 
for our intervals that satisfies the following three properties,
\begin{itemize}
\item \textbf{Local Dominance:}
For each interval $i \in [n]$,
there exists a bijection $\rho_i:\contain_i \rightarrow \{1, 2, \dots, \containn_i\}$
such that for all $j \in \contain_i$, $\assign_j \geq \rho_i(j)$.

\item \textbf{Global Dominance:}
For any decreasing and concave function $\bar\pen$,
$\sum_{i\in[n]} \bar\pen(\assign_i) \geq \sum_{i \in [n]} \bar\pen(\containn_i)$.
%the number of interval $i$ with $\containn_i \geq c$
%is at least 
%the number of interval $i$ with $\assign_i \geq c$,
%i.e.,
%$
%|\{i\in[n]:\containn_i \geq c\}| \geq 
%|\{i\in[n]:\assign_i \geq c\}|
%$.

\item \textbf{Partition Monotonicity:}
$n$ intervals can be partition into $m$ subgroups $A_1, A_2, \dots, A_m$
for some integer $m$ such that 
for all $k \in [m]$,
$
\{\assign_i: i \in A_k\} 
= 
\{
1, 2, \dots, |A_k|
\}
$.
\end{itemize}
\end{definition}

\begin{algorithm}[t]
\caption{Interval Assignment Solver
}\label{alg:interval assignment}
\begin{algorithmic}[1]

\State Initialize an assignment vector
$\assign_i = 0$ for all $i \in [n]$.
\State Initialize a pointer vector 
$\pfather_i = -1$ for all $i \in [n]$. 

\State Initialize a pointer vector
$\pmother_i = -1$  for all $i \in [n]$.

\State Initialize the remaining interval set 
$\remaining = \{1, 2, \dots, n\}$,
define $\remainingcontain_i = \contain_i \cap \remaining$
and $\remainingcontainn_i = |\remainingcontain_i|$.
%and $\remainingcontainn_i = |\contain_i \cap \remaining|$.

\While{$\remaining$ is not empty}
\State \begin{varwidth}[t]{\linewidth}
Find the interval $i$ with the largest index 
in the remaining interval set $\remaining$
%	  \par
%\hskip\algorithmicindent  
where $\remainingcontainn_i$ is maximized, 
i.e., $i =\,%\{
\argmax_{i\in W} \{\remainingcontainn_i
%\}
\}$. 
%\par\hskip
\end{varwidth}
\vspace{+1mm}
\State \begin{varwidth}[t]{\linewidth}
Find the interval $j$ with the smallest index %left most starting point
in the remaining interval set $\remaining$
which
covers position $a_i$,
i.e., $j = \min \remainingcontain_i$.
\end{varwidth}
\vspace{+1mm}
\State Set $\assign_j = \remainingcontainn_i$ and $\pmother_j = i$.

\For{all $k \in [n] / \remaining$ such that 
$j \in \contain_{\pmother_k}$ and $\assign_k = \assign_j + 1$}
\State Set $\pfather_k = j$. 
\EndFor

\State  
%\begin{varwidth}[t]{\linewidth}
Remove interval $j$ from the remaining interval set $\remaining$ %, and update $C(t)$ 
%for all remaining interval $t$,\par
%\hskip\algorithmicindent  
i.e., set
$\remaining = \remaining / \{j\}$.
%$C(t) = \{\tpre \in R \given 
%\tpre \leq t, f(\tpre) \geq t\}$.
%\end{varwidth}
\EndWhile
\State Return $\{\assign_1, \dots, \assign_n\}$.
\end{algorithmic}
\end{algorithm}

\begin{lemma}
For any input instance,
the solution of Interval Assignment Problem exists. Specifically, 
\Cref{alg:interval assignment} outputs such a solution.
\end{lemma}

\begin{proof}
In each iteration, \Cref{alg:interval assignment} 
pins down the assignment for a remaining interval and then remove it.
Thus, the algorithm terminates and outputs an assignment $\{\assign_1, \dots, \assign_n\}$.
We next show this assignment satisfies \emph{Local Dominance}, \emph{Global Dominance}
and \emph{Partition Monotonicity} separately.

\noindent\emph{\rom{1}. Local Dominance.}
%\paragraph{Local Dominance} 
For each interval $i \in [n]$,
consider $j_1, j_2, \dots \in \contain_i$ in the order which they are
removed from the algorithm:
for the $k$-th removed interval $j_k \in \contain_i$,
at that time $\remainingcontainn_i$ is $\containn_i - k + 1$,
which guarantees that $\assign_{j_k}$ is at least $\containn_i - k + 1$.
Thus, \emph{Local Dominance} is satisfied.

\noindent\emph{\rom{2}. Global Dominance.}
%\paragraph{Global Dominance}
We prove this by induction. Consider the reverse order of intervals removed
from the remaining interval set $\remaining$ in the algorithm,
i.e., we set $\remaining = \emptyset$ as the base case and then add intervals back to $\remaining$
in the reverse order which they have been removed in the algorithm. 
Our induction hypothesis is that restrict to intervals in $\remaining$,
\emph{Global Dominance} holds,
i.e., for any decreasing and concave function $\bar\pen$,
\begin{align}
\label{eq:global dominance}
\sum_{i\in \remaining} \bar\pen(\assign_i) \geq \sum_{i \in \remaining} \bar\pen(\remainingcontainn_i).
\end{align}

\emph{Base Case ($\remaining = \emptyset$):} In this case, the induction hypothesis holds trivially.

\emph{Inductive Step:}  Suppose the induction hypothesis holds before we add interval $i$ 
with $\assign_{i}$ back
to $\remaining$. 
Let $m = \assign_{i} - 1$.
To make it clear, let $\remaining$ to be the remaining interval set before we add interval $i$,
and $\remaining'$ to be the remaining interval set after we add interval $i$, i.e., 
$\remaining' = \remaining \cup\{i\}$.
%Let $\assign^{-1}(c) = |\{j \in W: \assign_j = c\}|$
%and 
%$\containn^{-1}(c) = |\{j \in W: |\contain_j \cap W| = c\}|$.
Next we consider the increment of both sides in 
\eqref{eq:global dominance}
after 
we add interval $i$ into $\remaining$.
The left hand side of \eqref{eq:global dominance} increases by $\bar\pen(m + 1)$.
%$\assign^{-1}(k)$ increases by one 
%while $\assign^{-1}(k')$ does not change for all $k' \not=k$.
For the right side, since $\assign_i = m + 1$,
there exist $m$ intervals $j_1, j_2, \dots j_m \in \remaining$
which 
%such that interval $j_k$ 
cover position $a_{\pmother_i}$,
and $i < j_k$ (otherwise, $j_k$ should be removed early than $i$ in the algorithm)
for all $k\in[m]$.
This implies that interval $i$ covers position $a_{j_k}$ 
for all $k \in[m]$.
Without loss of generality, we assume $j_1 < j_2 < \dots < j_m$,
then $\remainingcontainn_{j_k} \geq k$.
Hence, once we add interval $i$ into $W$,
the right hand side of \eqref{eq:global dominance}
increases by 
\begin{align*} &
\bar\pen(\containn_i^{\remaining'}) + 
\sum_{j\in \remaining}
\left(
\bar\pen(\containn_{j}^{\remaining'}) - 
\bar\pen(\remainingcontainn_{j})
\right) \\
\leq&\bar\pen(\containn_i^{\remaining'}) + 
\sum_{k\in[m]}
\left(
\bar\pen(\containn_{j_k}^{\remaining'}) - 
\bar\pen(\remainingcontainn_{j_k})
\right) \\
=&
\bar\pen(\containn_i^{\remaining'}) + 
\sum_{k\in[m]}
(\bar\pen(\remainingcontainn_{j_k} + 1) - 
\bar\pen(\remainingcontainn_{j_k})) \\ 
\overset{(a)}{\leq} &
\bar\pen(1) + 
\sum_{k \in [m]}
(
\bar\pen(k + 1) - \bar\pen(k)
) 
= \bar\pen(m + 1)
\end{align*}
where (a) holds because $\bar\pen$ is decreasing and concave.
Applying the induction hypothesis (before we add interval $i$),
the induction hypothesis (after we add interval $i$) holds,
which finishes the induction.

\noindent\emph{\rom{3}. Partition Monotonicity.}
%\paragraph{Partition Monotonicity}
We first introduce the following two claims:
(a) for each interval $i\in[n]$, there is at most one interval $j$ such that
$\pfather_j = i$;
(b) for each interval $i\in[n]$ with $\assign_i > 1$, $\pfather_i \not= -1$.  
Notice that claim (a) and (b) together imply that $\{\pfather_1, \dots, \pfather_n\}$ 
defines a partition which satisfies \emph{Partition Monotonicity} as follows:
\begin{enumerate}
\item[(i)] find an interval $i$ 
which is not in any current subgroups
and $\pfather_j \not= i$ for all $j\in[n]$
(halt if such interval $i$ does not exist)
\item[(ii)] create a new subgroup $A$,
\item[(iii)] while $\pfather_i \not= -1$, add interval $i$ into $A$, set $i = \pfather_i$, while end.
\item[(iv)] back to step (i).
\end{enumerate}
Next, we show claim (a) and claim (b) separately.

We show claim (a) by contradiction. 
Suppose there exists interval $i$, $j_1$ and $j_2$ such that 
$\pfather_{j_1} = \pfather_{j_2} = i$.
By the construction of the algorithm,
$\assign_{j_1} = \assign_{j_2} = \assign_i + 1$.
Now, consider case by case.
\begin{itemize}
\item \emph{Case 1 ($i < j_1$ or $i < j_2$):} Without loss of generality, we assume $i < j_1$,
and the case $i < j_2$ is symmetric.
%Consider the moment when the algorithm 
%removes interval $j_1$ due to $\pmother_{j_1}$.
By the construction of the algorithm,
$\pfather_{j_1} = i$ implies 
$i \in \contain_{\pmother_{j_1}}$. 
%interavl $i$ also covers position $a_{\pmother_{j_1}}$,
This leads to a contradiction, because 
if $i < j_1$, interval $i$ should be removed early than interval $j_1$ in the algorithm 
which implies $\assign_i \geq \assign_{j_1}$.
\item \emph{Case2 ($j_1, j_2 < i$):}
\begin{itemize}
\item \emph{Case 2a ($\pmother_{j_1} < \pmother_{j_2}$ or $\pmother_{j_2} < \pmother_{j_1}$):}
Without loss of generality, we assume $\pmother_{j_1} < \pmother_{j_2}$
and the case $\pmother_{j_2} < \pmother_{j_1}$ is symmetric.
\begin{itemize}
\item \emph{Case 2a1 (interval $j_1$ is removed before interval $j_2$):}
In this case, consider the moment 
when the algorithm removes $j_1$ due to interval $\pmother_{j_1}$.
By the construction of the algorithm, since $j_1$ is removed before $j_2$,
it implies
$\remainingcontainn_{\pmother_{j_1}} > \remainingcontainn_{\pmother_{j_2}}$.
Thus,
$\assign_{j_1}$ is strictly larger than $\assign_{j_2}$,
contradiction.
\item \emph{Case 2a2 (interval $j_2$ is removed before interval $j_1$):}
In this case, consider the moment 
when the algorithm remove $j_2$ due to interval $\pmother_{j_2}$.
Notice that interval $j_2$ also covers position $a_{\pmother_{j_1}}$,
i.e., $j_2 \in \contain_{\pmother_{j_1}}$.
By the construction of the algorithm, since $j_2$ is removed before $j_1$,
it implies
$\remainingcontainn_{\pmother_{j_1}}  \leq \remainingcontainn_{\pmother_{j_2}}$.
Thus, once the algorithm removed $j_2$, 
$\containn_{\pmother_{j_1}}^{\remaining/\{j_2\}}$ (which is an upper bound
of $\assign_{j_1}$) 
becomes strictly smaller than 
$\remainingcontainn_{\pmother_{j_2}}$ (which is equal to $\assign_{j_2}$), %which 
%implies $\assign_{j_1}$ is strictly smaller than $\assign_{j_2}$,
contradiction.
\end{itemize}

\item \emph{Case 2b ($\pmother_{j_1} = \pmother_{j_2}$):}
Without loss of generality, we assume interval $j_1$ is removed before interval $j_2$,
and the case where interval $j_2$ is removed before interval $j_1$ is 
symmetric.
Let $\pmother^* = \pmother_{j_1} = \pmother_{j_2}$. Consider the moment
when the algorithm removes $j_1$ due to $\pmother^*$.
By the construction of the algorithm,
$\assign_{j_1} = \remainingcontainn_{\pmother^*}$
and $\assign_{j_2} \leq \containn_{\pmother^*}^{\remaining/\{j_1\}} 
= \remainingcontainn_{\pmother^*} - 1$.
Thus, $\assign_{j_1}$ is strictly larger than $\assign_{j_2}$,
contradiction.
\end{itemize}
\end{itemize}

We show claim (b) as follows. For any interval $i$
with $\assign_i > 1$,
consider the next removed interval $j$ %which covers 
%position $a_{q_i}$ and is the first interval removed 
among
$\contain_{\pmother_i}$ after the algorithm removes interval $i$.
It is sufficient to show $\assign_j = \assign_i - 1$,
which implies that algorithm set $\pfather_i = j$ when it removes interval $j$.
Since $j$ is the next interval removed among $\contain_{\pmother_i}$ after 
interval $i$, $\assign_i - 1\leq \assign_j \leq \assign_i$.
To show $\assign_j < \assign_i$, we use contradiction.
Suppose $\assign_j = \assign_i$. If $i\in\contain_{\pmother_j}$,
this implies that at the moment when the algorithm removes $i$, 
$
\assign_i = \containn_{\pmother_i}^{\remaining}
\geq
\containn_{\pmother_j}^{\remaining} \geq \assign_j + 1 = \assign_i + 1
$, contradiction.
If $i \not\in \contain_{\pmother_j}$, since $i < j$, 
it implies that $\pmother_i < \pmother_j$ and
at the moment when the algorithm removes $i$,
$\containn_{\pmother_i}^\remaining
=
\assign_i
=\assign_j 
\leq \containn_{\pmother_j}^\remaining
$, contradiction.
\qedhere
\end{proof}

We present the formal proof of \Cref{thm:concave competitive ratio} below.

\begin{proof}[Proof of \Cref{prop:concave competitive ratio-iid}]
We start with the offline expected LP on the reverse type sequence, i.e., $\EAR{\inversetypesequence}$
where $\type_t' = \type_{\totaltime - t + 1}$,
\begin{align*}
%\nonumber
&\begin{array}{rlll}
\max
\limits_{\mathbf \alloc \geq \mathbf 0} &
\displaystyle\sum\nolimits%\limits
_{t=1}^\totaltime
\displaystyle\sum\nolimits%\limits
_{\assortment \in \assortmentspace}
\displaystyle\sum\nolimits%\limits
_{i=1}^n
\reward_i\curchoice\curalloc
&
\text{s.t.}
&\\ %& & &\\
&
\displaystyle\sum\nolimits_{\tpre = t}^{\totaltime}
\displaystyle\sum\nolimits_{\assortment \in \assortmentspace}
%(1-\durationdistribution_i(t - \tpre)) 
%\prob[\durationdistribution_i]{\duration_{i,\tpre} \geq \tpre - t}
\durationcdfi_i(\tpre - t)
\prechoice\prealloc \leq \inventory_i
& i \in [n],\ t \in [\totaltime]
%\forall i\in[n],t \in [T] 
&\langle\inventorydual\rangle
\\
&\displaystyle\sum\nolimits_{\assortment\in \assortmentspace}\curalloc \leq 1
&t \in [\totaltime]
&\langle\probdual\rangle \\
%\end{array}\\
\intertext{We construct its dual program with dual variable $\inventorydual$ 
and $\probdual$ as follows,} 
%\nonumber
%	&\begin{array}{rlll}
\min
\limits_{\boldsymbol{\theta},\boldsymbol{\lambda} \geq \mathbf 0} &
\displaystyle\sum\nolimits%\limits
_{t=1}^\totaltime
\displaystyle\sum\nolimits%\limits
_{i=1}^n
\inventory_i\inventorydual
+
\displaystyle\sum\nolimits_{t =1}^\totaltime
\probdual
& 
\text{s.t.} 
&\\ %& & &\\
&
\probdual + 
\displaystyle\sum\nolimits_{i = 1}^n
\displaystyle\sum\nolimits_{\tpre= 1}^t
%(1-\durationdistribution_i(t - \tpre)) 
%\prob[\durationdistribution_i]{\duration_{i,\tpre} \geq t - \tpre}
\durationcdfi_i(t - \tpre)
\curchoice\theta_{i,\tpre}
%& & \\
%				&  
%		\qquad\qquad
%		\qquad\qquad
%		\qquad\qquad
%		\qquad\qquad
\geq \displaystyle\sum\nolimits_{i = 1}^n
\reward_i\curchoice
& \assortment \in \assortmentspace,\ t \in [\totaltime]
%\forall i\in[n],t \in [T] 
&\langle\curalloc\rangle
\end{array}
\end{align*}	
Let $\assortment_t$ be the assortment offered to consumer $t$.
Recall $\curinventorya$ 
%(resp.\ $\curinventoryb$) 
is the 
inventory level of product $i$ at time period $t$ 
before 
%(resp.\ after) 
the realization of 
consumer selection. 
For each product $i$,
consider the following 
instance of the Interval Assignment Problem (IAP)
in \Cref{def:IAP}
separately.
Let 
%it has been allocated at time 
$\texttt{alloc}_i = \{t_1, t_2, \dots, t_m\}$
be the time periods when product $i$ is selected,
and let 
the correpsonding rental duration of product $i$ be 
$d_{t_1}, d_{t_2}, \dots, d_{t_m}$, respectively.
Let the instance of IAP with $m$ intervals,
where each interval $[t_j, t_j + d_{t_j}]$ corresponds to 
the event that a unit of product $i$ has been selected 
by a consumer at time $t_j$ and returned to the platform 
at time $t_j + d_{t_j}$.
Let 
$\{\assign_{i, t}\}_{t\in \texttt{alloc}_i}$ 
be the assignment solved in IAP for product $i$ 
and let 
$\pseudoinventory_{i, t} = \inventory_i - \assign_{i, t}$ if $t \in \texttt{alloc}_i$
and $\pseudoinventory_{i, t} = 1$ otherwise.
Consider the following assignments for primal 
of (forward) expected LP, 
and dual 
of the reverse expected LP,
\begin{align*}
\textit{Primal:}~~~~~\curalloc &= \indicator{\assortment_t = \assortment},\\
\textit{Dual:}~~~~~~~ \probdual &= \displaystyle\sum\nolimits_{i = 1}^n \reward_i 
\pen\left(\frac{\curinventorya}{\inventory_i}\right)
\cdot
\indicator{\text{product $i$ is selected at time $t$}},\\
~~~~~~~~\inventorydual &= \reward_i\left(
\pen\left(\frac{\curpseudoinventory}{\inventory_i}\right) -
\pen\left(\frac{\curpseudoinventory - 1}{\inventory_i}\right)
\right) 
\cdot
\indicator{\text{product $i$ is selected at time $t$}}
\end{align*}
where 
$\indicator{\cdot}$ is an indicator operator. Note that product $i$ is selected at time $t$ if it belongs to the assortment set $\assortment_t$ and consumer arriving at time $t$ chooses this product.  In the rest of analysis, we show that the above primal assignment is feasible in the primal of forward expected LP, the above randomized dual assignment is feasible in expectation in the dual of reverse  expected LP, and finally the expected objective value of primal is at least $\alpha= \GNRnotation$ fraction of the expected objective value of the dual. Similar to  \Cref{lem:random primal-dual}, satisfying these properties is enough to finish the proof.
\vspace{1mm}

%Construct 
%the following solution of primal and dual,
%\begin{align*}
%	\curalloc &= 
%	\indicator{\assortment_t = \assortment},
%\left\{
%\begin{array}{ll}
%	1 \qquad & \text{if } \assortment = \assortment_t \\
%	0 & \text{otherwise.}
%\end{array}
%\right. 
%\;\;\;
%\;\;\;
%\qquad\qquad
%\qquad\qquad
%\qquad\quad
%	\probdual 
%	= 
%\displaystyle\sum\nolimits_{i = 1}^n \reward_i \choice^{\type_t}(\assortment_t, i)\curpena
%	\displaystyle\sum\nolimits_{i = 1}^n \reward_i 
%	\pen\left(\frac{\curinventorya}{\inventory_i}\right)
%	\cdot
%	\indicator{\text{product $i$ is selected at time $t$}},
%	\\ %\mbox{and}\;\;
%	\inventorydual &= \reward_i\left(
%	\pen\left(\frac{\curpseudoinventory}{\inventory_i}\right) -
%	\pen\left(\frac{\curpseudoinventory - 1}{\inventory_i}\right)
%\right) 
%\cdot
%\indicator{\text{product $i$ is selected at time $t$}}
%																								\end{align*}
%where 
%$\indicator{\text{product $i$ is selected at time $t$}}$ is the indicator
%variable that consumer selects product $i$ at time $t$,
%and 
%$\indicator{\assortment_t = \assortment}$
%is the indicator variable that assortment $\assortment$ is offered at time $t$.

%\paragraph{Feasibility of primal solution}
%Due to the property of Inventory-Balancing, i.e., $S_t$ offered by IB is always
%inventory feasible, the primal solution is feasible.

\noindent\emph{\rom{1}. Primal feasibility and dual feasibility in expectation.}
The primal assignment is feasible, 
as Inventory-Balancing only offers inventory feasible assortments. 
To show dual feasibility in expectation, 
first note that $\pen(.)$ is non-negative and monotone non-decreasing. 
Therefore $\probdual\geq 0$ for all $t\in[\totaltime]$, 
and $\inventorydual\geq 0$ for all $i\in[n],t\in[\totaltime]$. 
Next, we show for every $t\in[\totaltime]$ and $\assortment\in\assortmentspace$, 
the dual assignment satisfies the dual constraints 
corresponding to $\curalloc$ in expectation. 
Let $\indicator{\duration_{i,\tpre} \geq t - \tpre}$ be the indicator 
of the event that rental time of product $i$ at time $\tpre$ is at least 
$t - \tpre$. For every product $i\in[n]$, the following inequality holds at every time $t\in[\totaltime]$: 
%
%\paragraph{Feasibility of expected dual solution}
%To see that the dual solution is feasible in expectation, 
%let $\indicator{\duration_{i,\tpre} \geq t - \tpre}$ be the indicator variable 
%that the rental duration of product $i$ at time $\tpre$ is at least 
%$t - \tpre$.
%We first show that the following inequality holds for all product $i$, 
%all time $t$ and all realization,
\begin{align}
\label{eq:dual feasible ex post concave}
\reward_i\pen\left(\frac{\curinventorya}{\inventory_i}\right) 
+ \displaystyle\sum\nolimits_{\tpre = 1}^{t - 1}
\indicator{\duration_{i,\tpre} \geq t - \tpre} \cdot
\theta_{i, \tpre} 
\geq \reward_i
\end{align}
To see why inequality~\eqref{eq:dual feasible ex post concave} holds, 
consider on-hand units and under rental units of product $i$ at time $t$. 
Since the inventory level of product $i$ at time $t$  is 
$\curinventorya$, 
there are $\inventory_i - \curinventorya$ units of product $i$ 
under rental at that moment. Suppose these units were rented at times
$\tpre_1, \tpre_2, \dots, \tpre_{\inventory_i - \curinventorya}$,
where $\indicator{d_{\tpre_j} \geq t - \tpre_j} = 1$ and 
$\indicator{\text{product $i$ is selected at time $\tpre_j$}} = 1$
for all $j\in[\inventory_i - \curinventorya]$.
Additionally, recall 
$\{\assign_{i, t}\}_{t\in \texttt{alloc}_i}$ is assignment in IAP which satisfies
\emph{Local Dominance}.
%Consider interval start at 
%$\tpre_{\inventory_i - \curinventorya}$.
%$[\tpre_{\inventory_i - \curinventorya}, \tpre_{\inventory_i - \curinventorya} + 
%\duration_{i,\tpre_{\inventory_i - \curinventorya}}]$.
By Local Dominance at interval starting at $\tpre_{\inventory_i - \curinventorya}$,
there exists a bijection $\rho$ from $\contain_{\tpre_{\inventory_i - \curinventorya}}$
to $\{1,2,\dots,\containn_{\tpre_{\inventory_i - \curinventorya}}\}$ such that 
$\assign_{\tpre} \geq \rho(\tpre)$ for all $\tpre \in \contain_{\tpre_{\inventory_i - \curinventorya}}$.
Notice that intervals starting at 
$\tpre_1, \tpre_2, \dots \tpre_{\inventory_i - \curinventorya}$
all cover time $\tpre_{\inventory_i - \curinventorya}$,
i.e.,
$\tpre_j \in \contain_{\tpre_{\inventory_i - \curinventorya}}$ for all 
$j\in[\inventory_i - \curinventorya]$.
This implies there exists another bijection $\rho'$ from
$[\inventory_i - \curinventorya]$
to $[\inventory_i - \curinventorya]$
such that
$\assign_{\tpre_j} \geq \rho'(j)$
for all $j \in [\inventory_i - \curinventorya]$.
Because the penalty function $\pen(\cdot)$ is concave and increasing,
\begin{align}
\begin{split}
\label{eq:concave concave}
\theta_{i, \tpre_j} &= 
\reward_i\left(\pen\left(\frac{\pseudoinventory_{i, \tpre_j}}{\inventory_i}\right)
-
\pen\left(\frac{\pseudoinventory_{i, \tpre_j} - 1}{\inventory_i}\right)\right)  \\
&=
\reward_i\left(\pen\left(\frac{\inventory_i - \assign_{i, \tpre_j}}{\inventory_i}\right)
-
\pen\left(\frac{\inventory_i - \assign_{i, \tpre_j} - 1}{\inventory_i}\right)\right)  \\
&\geq
\reward_i\left(\pen\left(\frac{\inventory_i - \rho'(j)}{\inventory_i}\right)
-
\pen\left(\frac{\inventory_i - \rho'(j) - 1}{\inventory_i}\right)\right)
\end{split}
\end{align}
By applying \eqref{eq:concave concave}, 
we can prove inequality~\eqref{eq:dual feasible ex post concave}:
\begin{align*}
&\quad~\reward_i\pen\left(\frac{\curinventorya}{\inventory_i}\right) 
+ \displaystyle\sum\nolimits_{\tpre = 1}^{t - 1}
\indicator{\duration_{i, \tpre} \geq t - \tpre} \cdot
\theta_{i, \tpre}\\
& =\reward_i\pen\left(\frac{\curinventorya}{\inventory_i}\right) 
+ \displaystyle\sum\nolimits_{j = 1}^{\inventory_i - \curinventorya} \reward_i
\left(\pen\left(\frac{\pseudoinventory_{i, \tpre_j}}{\inventory_i}\right)
-
\pen\left(\frac{\pseudoinventory_{i, \tpre_j} - 1}{\inventory_i}\right)\right)\\
&\geq \reward_i\pen\left(\frac{\curinventorya}{\inventory_i}\right) + \displaystyle\sum\nolimits_{j = 1}^{\inventory_i - \curinventorya} \reward_i\left(\pen\left(\frac{\inventory_i - \rho'(j)}{\inventory_i}\right)
-
\pen\left(\frac{\inventory_i - \rho'(j) - 1}{\inventory_i}\right)\right)\\
&=\reward_i\pen\left(\frac{\curinventorya}{\inventory_i}\right) +\displaystyle\sum\nolimits_{I = \curinventoryb}^{\inventory_i - 1} 
\reward_i\left(
\pen\left(\frac{I}{\inventory_i}\right) 
-
\pen\left(\frac{I-1}{\inventory_i}\right) 
\right)\\
&=
\pen\left(\frac{\inventory_i - 1}{\inventory_i}\right) 
+
\pen\left(\frac{\curinventorya}{\inventory_i}\right) 
-
\pen\left(\frac{\curinventorya-1}{\inventory_i}\right) 
\geq\reward_i\pen(1)=\reward_i
\end{align*}

Now, for each time $t\in[\totaltime]$ and assortment $\assortment\in\assortmentspace$, consider the following expression:
\begin{align}
\label{eq:dual LHS concave}
\probdual + 
\displaystyle\sum\nolimits_{i = 1}^n\displaystyle\sum\nolimits_{\tpre = 1}^t
\indicator{\duration_{i, \tpre} \geq t - \tpre}
\curchoice \theta_{i, \tpre} 
\end{align}
On the one hand, note that by taking expectation from \eqref{eq:dual LHS concave} we have 
\begin{equation}
\label{eq:first-compare concave}
\expect{\probdual + 
\displaystyle\sum\nolimits_{i = 1}^n\displaystyle\sum\nolimits_{\tpre = 1}^t
\indicator{\duration_{i, \tpre} \geq t - \tpre}
\curchoice \theta_{i, \tpre} }=\expect{\probdual} + 
\displaystyle\sum\nolimits_{i = 1}^n\displaystyle\sum\nolimits_{\tpre = 1}^t
\durationcdfi_i(t - \tpre)
\curchoice\expect{ \theta_{i, \tpre}}~,
\end{equation}
simply because $\theta_{i, \tpre}$ and $\indicator{\duration_{i, \tpre} \geq t - \tpre}$ are independent random variables (as rental time $\duration_{i, \tpre}$ is realized independently from the assortment and the consumer's selection at any time $\tpre$). On the other hand, by taking expectation from 
\eqref{eq:dual LHS concave} first over the randomness in the choice of consumer at time $t$, i.e., by conditioning on (i) history up to time $t$ (including rental times $\{\duration_{i, \tpre}\}_{\tpre=1}^{t-1}$ and the inventory levels $\curinventorya$ for each product $i$), and (ii) assortment $\assortment_t$ offered at time $t$, we have
%(notice that this is independent of all events before $t$ or 
%the assortment $\assortment_t$ offered at time $t$ or 
%the inventory level at time $t$),
\begin{align}
&\expect{\probdual + 
\displaystyle\sum\nolimits_{i = 1}^n\displaystyle\sum\nolimits_{\tpre = 1}^t
\indicator{\duration_{i, \tpre} \geq t - \tpre}
\curchoice \theta_{i, \tpre} |\mathcal{F}_{t-1},\assortment_t}\nonumber\\
=&\displaystyle\sum\nolimits_{i = 1}^n 
\reward_i\choice^{\type_t}(\assortment_t, i)
\pen\left(\frac{\curinventorya}{\inventory_i}\right)
+	
\displaystyle\sum\nolimits_{i = 1}^n\displaystyle\sum\nolimits_{\tpre = 1}^{t - 1}
\indicator{\duration_{i, \tpre} \geq t - \tpre}
\curchoice \theta_{i, \tpre} \nonumber \\
&+
\displaystyle\sum\nolimits_{i = 1}^n 
\choice^{\type_t}(\assortment, i)\reward_i
\choice^{\type_t}(\assortment_t, i)
\left(
\pen\left(\frac{\curpseudoinventory}{\inventory_i}\right)
-
\pen\left(\frac{\curpseudoinventory - 1}{\inventory_i}\right)
\right)\label{eq:third-term concave}\\
\overset{(a)}{\geq} &
\displaystyle\sum\nolimits_{i = 1}^n 
\reward_i\curchoice
\pen\left(\frac{\curinventorya}{\inventory_i}\right)
+	
\displaystyle\sum\nolimits_{i = 1}^n\displaystyle\sum\nolimits_{\tpre = 1}^{t - 1}
\indicator{\duration_{i, \tpre} \geq t - \tpre}
\curchoice \theta_{i, \tpre}\nonumber  \\
=&\displaystyle\sum\nolimits_{i = 1}^n 
\curchoice\left(\reward_i\pen\left(\frac{\curinventorya}{\inventory_i}\right)+ \displaystyle\sum\nolimits_{\tpre = 1}^{t - 1}
\indicator{\duration_{i, \tpre} \geq t - \tpre} \cdot
\theta_{i, \tpre}  \right)
\nonumber \\
\overset{(b)}{\geq}& \displaystyle\sum\nolimits_{i = 1}^n 
\reward_i\curchoice~,\nonumber
\end{align}
where $\mathcal{F}_{t-1}$ denotes the history up to time $t$. Note that inequality~(a) above holds because $$
\assortment_t = 
\argmax_{\assortment \in \assortmentspace}\displaystyle\sum\nolimits_{i = 1}^n\reward_i\curchoice
\pen\left(\frac{\curinventorya}{\inventory_i}\right)~,
$$
and the third term in expression~\eqref{eq:third-term concave} is non-negative, and inequality~(b) holds because of  inequality~\eqref{eq:dual feasible ex post concave}. Therefore, by taking full expectation we have
\begin{equation}
\label{eq:second-compare concave}
\expect{\probdual + 
\displaystyle\sum\nolimits_{i = 1}^n\displaystyle\sum\nolimits_{\tpre = 1}^t
\indicator{\duration_{i, \tpre} \geq t - \tpre}
\curchoice \theta_{i, \tpre} }\geq \displaystyle\sum\nolimits_{i = 1}^n 
\reward_i\curchoice
\end{equation}
Combining \eqref{eq:first-compare concave} and \eqref{eq:second-compare concave} shows feasibility in expectation of the dual assignment.
%	\begin{align}
%		\label{eq:dual feasible ex post final}
%		\eqref{eq:feasibility ex post} 
%		\geq 
%		\displaystyle\sum\nolimits_{i = 1}^n 
%		\reward_i\curchoice
%		\pen\left(\frac{\curinventorya}{\inventory_i}\right)
%		&+	
%		\displaystyle\sum\nolimits_{i = 1}^n\displaystyle\sum\nolimits_{\tpre = 1}^{t - 1}
%		\indicator{\duration_{i, \tpre} \geq t - \tpre}
%		\curchoice \theta_{i, \tpre}  
%	\end{align}
%	Applying inequality \eqref{eq:dual feasible ex post}, it implies
%	\begin{align*}
%		\eqref{eq:feasibility ex post} 
%		\geq 
%		\displaystyle\sum\nolimits_{i = 1}^n 
%		\reward_i\curchoice.
%	\end{align*}
%	where $
%		\displaystyle\sum\nolimits_{i = 1}^n 
%		\reward_i\curchoice$
%		is the right hand side of the dual constraint corresponding to the
%		primal variable $\curalloc$.
%	Having this inequality,

\vspace{1mm}

\noindent\emph{\rom{2}. Comparing objective values of primal and dual.}
%By the fact that $\frac{A + B}{C + D} \geq \min\{\frac{A}{C} , \frac{B}{D}\}$,
We consider the contribution of each product $i$ in primal and dual 
(i.e. $\text{Primal}_{i}$ and $\text{Dual}_{i}$)
at each realization 
separately.
%The contributions of product in primal and dual for any fixed realization
%are as follows, 
Recall $\texttt{alloc}_i$ is the set of time periods when
a unit of product $i$ has been selected,
\begin{align*}
\text{Primal}_i &= 
\reward_i
%\left(
\displaystyle\sum\nolimits_{t = 1}^\totaltime
\indicator{\text{product $i$ is selected at time $t$}}
%\right)
\\
&= \reward_i|\texttt{alloc}_i| \\
\text{Dual}_i &= 
\reward_i
\displaystyle\sum\nolimits_{t = 1}^\totaltime 
\left(
\pen\left(\frac{\curinventorya}{\inventory_i}\right) 
+
\inventory_i\left(\pen\left(\frac{\curpseudoinventory}{\inventory_i}\right) 
-
\pen\left(\frac{\curpseudoinventory - 1}{\inventory_i}\right) \right)
\right)
\indicator{\text{product $i$ is selected at time $t$}} \\
&=
\reward_i
\displaystyle\sum\nolimits_{t \in \texttt{alloc}_i} 
\left(
\pen\left(\frac{\curinventorya}{\inventory_i}\right) 
+
\inventory_i\left(
\pen\left(\frac{\curpseudoinventory}{\inventory_i}\right) 
-
\pen\left(\frac{\curpseudoinventory - 1}{\inventory_i}\right) \right)
\right)
\end{align*}
Consider decreasing and concave function $\bar\pen(x) = \pen(1 - x)$,
by \emph{Global Dominance} of IAP assignment,
\begin{align*}
\sum_{t\in \texttt{alloc}_i}
	\pen\left(\frac{\curpseudoinventory}{\inventory_i}\right)  
	&=
\sum_{t\in \texttt{alloc}_i}
	\pen\left(\frac{\inventory_i - \assign_{i, t}}{\inventory_i}\right)   
	=
\sum_{t\in \texttt{alloc}_i}
\bar\pen\left(\frac{ \assign_{i,t}}{\inventory_i}\right)  
\geq 
\sum_{t\in \texttt{alloc}_i}
\bar\pen\left(\frac{\inventory_i - \curinventorya}{\inventory_i}\right)  
	=
\sum_{t\in \texttt{alloc}_i}
	\pen\left(\frac{\curinventorya}{\inventory_i}\right)   
\intertext{Hence,}
\text{Dual}_i &\leq 
\reward_i
\displaystyle\sum\nolimits_{t \in \texttt{alloc}_i} 
\left(
\pen\left(\frac{\curpseudoinventory}{\inventory_i}\right) 
+
\inventory_i\left(
\pen\left(\frac{\curpseudoinventory}{\inventory_i}\right) 
-
\pen\left(\frac{\curpseudoinventory - 1}{\inventory_i}\right) \right)
\right)
\end{align*}
Now, we partition time periods in $\texttt{alloc}_i$ into subgroups $A_{i, 1}, A_{i, 2}, \dots, A_{i, m}$ 
defined by \emph{Partition Monotonicity}
of IAP assignment, and consider the contribution of each subgroup $A_{i, k}$ in primal and dual 
(i.e. $\text{Primal}_{A_{i, k}}$ and $\text{Dual}_{A_{i, k}}$)
separately.
Recall that \emph{Partition Monotonicity} guarantees that 
$\{\assign_{i, t}:t \in A_{i, k}\} = \{1, 2, \dots, |A_{i, k}|\}$,
thus,
$\{\curpseudoinventory:t \in A_{i, k}\} 
= \{\inventory_i - |A_{i, k}| + 1, \inventory_i - |A_{i, k}| + 2, \dots, \inventory_i\}$.
Thus, let $x = \frac{\inventory_i - |A_{i, k}|}{\inventory_i}$,
\begin{align*}
\text{Primal}_{A_{i, k}} &= \reward_i \inventory_i (1-x) \\
\text{Dual}_{A_{i, k}} 
&\leq 
\reward_i \sum_{I = \inventory_i x + 1}^{\inventory_i}
\left(
\pen\left(\frac{I}{\inventory_i}\right) 
+
\inventory_i\left(
\pen\left(\frac{I}{\inventory_i}\right) 
-
\pen\left(\frac{I- 1}{\inventory_i}\right) \right)
\right) \\
&= 
\reward_i 
\sum_{I = \inventory_i x + 1}^{\inventory_i}
\pen\left(\frac{I}{\inventory_i}\right) 
+
\reward_i\inventory_i\left(
\pen(1) - 
\pen\left(x
%\frac{x}{\inventory_i}
\right)
\right)
\intertext{
Since $\pen(1) = 1$ and $\pen$ is increasing, it implies}
\sum_{I = \inventory_i x + 1}^{\inventory_i}
\pen\left(\frac{I}{\inventory_i}\right) 
&=
1 + 
\sum_{I = \inventory_i x + 1}^{\inventory_i - 1}
\pen\left(\frac{I}{\inventory_i}\right) \leq 
1 + 
\int_{x+\frac{1}{\inventory_i}}^1
\pen(y)\,dy
\intertext{
Thus,
}
\text{Dual}_{A_{i, k}} &\leq 
\reward_i\inventory_i\left(
\frac{1}{\inventory_i} + \int_{x+\frac{1}{\inventory_i}}^1
\pen(y)\,dy
+
1 -
\pen\left(
x
%\frac{x}{\inventory_i}
\right)
\right)
\intertext{and}
\frac{\text{Primal}_{A_{i, k}}}
{\text{Dual}_{A_{i, k}}} 
&\geq
\frac{1 - x}
{
\frac{1}{\inventory_i} + \int_{x+\frac{1}{\inventory_i}}^1
\pen(y)\,dy
+
1 -
\pen\left(
x
\right)
}
\end{align*}
Thus, we finish showing that 
\begin{align*}
\frac{\text{Primal}}
{\text{Dual}} 
&\geq
\min_{i \in [n]}
\frac{\text{Primal}_i}
{\text{Dual}_i}  
\geq
\min_{i \in [n]}
\min_{A_{i, k}}
\frac{\text{Primal}_{A_{i, k}}}
{\text{Dual}_{A_{i, k}}}   \\
&\geq
\GNRbound.
\end{align*}
Invoking \Cref{lem:random primal-dual} finishes the proof.
\end{proof}
